# Supplementary material for: Program Targeting with Machine Learning and Mobile Phone Data: Evidence from an Anti-Poverty Intervention in Afghanistan
Source: arXiv:2206.11400 source file (2022-06-22)
Supplement: Supplementary file 4 [file appendix_consumption.tex]

\begin{table}[H]
\centering
\footnotesize

\begin{tabular}{lllll}
\toprule
Targeting Method &           AUC &      Accuracy &     Precision &        Recall \\
\midrule

          Random &  0.50 (0.027) &  0.60 (0.025) &  0.27 (0.036) &  0.27 (0.036) \\
     Asset Index &  0.66 (0.025) &  0.68 (0.022) &  0.41 (0.040) &  0.41 (0.040) \\
   Ultra-Poverty &  0.62 (0.022) &  0.70 (0.021) &  0.45 (0.037) &  0.45 (0.037) \\
             CDR &  0.47 (0.028) &  0.58 (0.027) &  0.23 (0.036) &  0.23 (0.036) \\
\bottomrule
\end{tabular}
\caption{Replication of Table \ref{resultstable} Panel A with ``extreme poverty" as the ground truth measure of poverty, testing the extent to which each targeting method reaches the poorest 27\% of the 535-household matched sample by consumption. For CDR-predicted poverty, we retrain the gradient boosting classification model to predict extreme poverty.} 
\label{appendix:consumption} 
\end{table}
